# Supplementary material for: SEEV: Synthesis with Efficient Exact Verification for ReLU Neural Barrier Functions
Source: arXiv:2410.20326 source file (2024-10-27)
Supplement: Supplementary file 1 [file Supplement.tex]

% \newpage
\section{Supplementary Material}
In what follows, we give some details of content omitted in the paper due to space limit. The supplements are organized as follows. We give some proof of Lemma~\ref{lemma:activation-region}, \ref{lemma:NN-invariant}, Proposition~\ref{prop:safety-condition}, Lemma~\ref{lemma:single-activation-set-condition}, \ref{lemma:multi-activation-set-condition}, and Theorem~\ref{theorem:overall-verification-proof} in Section~\ref{proof:lemma:activation-region}
% \ref{proof:lemma:NN-invariant}\ref{proof:prop:safety-condition}\ref{proof:lemma:single-activation-set-condition}\ref{proof:lemma:multi-activation-set-condition}
--\ref{proof:theorem:overall-verification-proof}, respectively. We present system dynamics for Darboux, obstacle avoidance, spacecraft rendezvous and hi-ord$_8$ in Section \ref{sup:darboux}--\ref{sup:hi-ord}. We provide some training details in Section \ref{subsec:training_details} as well as experiment details and results in Section \ref{subsec:experiment_details}. We compare polynomial CBFs with NCBF in \ref{sup:NCBF_polyCBF}, compare NCBFs with different activation functions in \ref{sup:cmp_activation}. We present more details in \ref{sup:ce} on the example in \ref{subsec:safety-conditions}. 

\subsection{Proof of Lemma \ref{lemma:activation-region}}
\label{proof:lemma:activation-region}
We prove by induction on $L$. If $L=1$, then $x \in \overline{\mathcal{X}}(\mathbf{S})$ if the pre-activation input to the $(1,j)$ neuron is nonnegative for all $j \in S_{1}$ and nonpositive for all $j \notin S_{1}$. We have that the pre-activation input is equal to $W_{1j}^{T}x + r_{1j}$, establishing the result for $L=1$. 

Now, inducting on $L$, we have that $x \in \overline{\mathcal{X}}(S_{1},\ldots,S_{L-1})$ if and only if
\begin{multline*}
x \in \bigcap_{i=1}^{L-1}{\left(\bigcap_{j \in S_{i}}{\{x : W_{ij}^{T}(\overline{\mathbf{W}}_{i-1}(\mathbf{S})^{T}x + \overline{\mathbf{r}}_{i-1}) + r_{ij} \geq 0\} }\right.} \\
\left.
\cap \bigcap_{j \notin S_{i}}{\{x : W_{ij}^{T}(\overline{\mathbf{W}}_{i-1}(\mathbf{S})^{T}x + \overline{\mathbf{r}}_{i-1}) + r_{ij} \leq 0\}}\right)
\end{multline*}

by induction. If $x \in \overline{\mathcal{X}}(S_{1},\ldots,S_{L-1})$, then $x \in \overline{\mathcal{X}}(S_{L})$ if and only if the pre-activation input to the $j$-th neuron at layer $L$ is nonnegative for all $j \in S_{L}$ and nonpositive for $j \notin S_{L}$. The pre-activation input is equal to $W_{Lj}^{T}z_{L-1} + r_{Lj}$, which we can expand by induction as
\begin{eqnarray*}
    W_{Lj}^{T}z_{L-1} + r_{Lj} &=& \sum_{j^{\prime}=1}^{M_{L-1}}{(W_{Lj})_{j^{\prime}}z_{L-1,j^{\prime}}} + r_{Lj} \\
    &=& \sum_{j^{\prime}=1}^{M_{L-1}}{(W_{Lj})_{j^{\prime}}(\overline{\mathbf{W}}_{L-1,j^{\prime}}(\mathbf{S})^{T}x+\overline{\mathbf{r}_{L-1,j^{\prime}}}(\mathbf{S})} + r_{Lj} \\
    &=& \left(\sum_{j^{\prime}=1}^{M_{L-1}}{(W_{Lj})_{j^{\prime}}\overline{W}_{L-1,j^{\prime}}(\mathbf{S})}\right)^{T}x + \overline{\mathbf{r}}_{Lj}(\mathbf{S}) \\
    &=& (\overline{\mathbf{W}}_{L-1}(\mathbf{S})W_{Lj})^{T}x + \overline{\mathbf{r}}_{Lj}(\mathbf{S})
\end{eqnarray*}
completing the proof.

\subsection{Proof of Lemma \ref{lemma:NN-invariant}}
\label{proof:lemma:NN-invariant}

The proof approach is based on Nagumo's Theorem, which gives necessary and sufficient conditions for positive invariance of a set. We first define the concept of tangent cone, and then present positive invariance conditions based on the tangent cone. The approach of the proof is to characterize the tangent cone to the set $\mathcal{D} = \{x: b(x) \geq 0\}$. 

\begin{definition}
\label{def:tangent-cone}
Let $\mathcal{A}$ be a closed set. The tangent cone to $\mathcal{A}$ at $x$ is defined by
\begin{equation}
\label{eq:tangent-cone}
\mathcal{T}_{\mathcal{A}}(x) = \left\{z : \liminf_{\tau \rightarrow 0}{\frac{\mbox{dist}(x+\tau z, \mathcal{A})}{\tau}} = 0\right\}
\end{equation}
\end{definition}

The following result gives an approach for constructing the tangent cone.

\begin{lemma}[\cite{blanchini2008set}]
\label{lemma:TC-special}
Suppose that the set $\mathcal{A}$ is defined by $$\mathcal{A} = \{x: q_{k}(x) \leq 0, k=1,\ldots,N\}$$ for some collection of differentiable functions $q_{1},\ldots,q_{N}$. For any $x$, let $J(x) = \{k: q_{k}(x) = 0\}$. Then $$\mathcal{T}_{\mathcal{A}}(x) = \{z: z^{T}\nabla q_{k}(x) \leq 0 \ \forall k \in J(x)\}.$$
\end{lemma}

The following is a fundamental preliminary result for  establishing positive invariance.

\begin{theorem}[Nagumo's Theorem \cite{blanchini2008set}, Section 4.2]
\label{theorem:Nagumo}
A closed set $\mathcal{A}$ is controlled positive invariant if and only if, whenever $x(t) \in \partial \mathcal{A}$,  $u(t) \in \mathcal{U}$ satisfies
\begin{equation}
\label{eq:Nagumo-CPI}
(f(x(t)) + g(x(t))u(t)) \in \mathcal{T}_{\mathcal{A}}(x(t))
\end{equation}
\end{theorem}

The following lemma characterizes the tangent cone to $\mathcal{D}$.

\begin{proposition}
\label{lemma:tangent-cone-NN}
For any $x\in \partial\mathcal{D}$, we have 
\begin{multline}
\label{eq:tangent-cone-NN}
\mathcal{T}_{\mathcal{D}}(x) = 
\bigcup_{\mathbf{S} \in \mathbf{S}(x)}{\left[\left(\bigcap_{(i,j) \in \mathbf{T}(x) \cap \mathbf{S}}{\{z: (\overline{\mathbf{W}}_{i-1}(\mathbf{S})W_{ij})^{T}z \geq 0\}}\right) \cap \right.} \\
\left. \left(\bigcap_{(i,j) \in \mathbf{T}(x) \setminus \mathbf{S}}{\{z : (\overline{\mathbf{W}}_{i-1}(\mathbf{S})W_{ij})^{T}z \leq 0\}}\right) 
\cap  \{z : \overline{W}(\mathbf{S})^{T}z \geq 0\}\right]
\end{multline}
\end{proposition}

\begin{proof}%[Proof of Proposition \ref{prob:CPI}]
%As a preliminary, we show that when $x \in D_{i}$, $\mathcal{T}_{\Psi_{i}}(x) = \mathcal{T}_{\mathcal{C}}(x)$. Indeed, by Lemma \ref{lemma:curve-boundary-intersection}, $D_{i}$ is a connected component of the boundary of $\mathcal{C}_{0}$ and hence a connected component of $\partial \mathcal{C}_{0}$. Hence $\mbox{dist}(x + \tau z,\mathcal{C}) = \mbox{dist}(x + \tau z, \Psi_{i})$ for $\tau$ sufficiently small, implying that $z \in \mathcal{T}_{\mathcal{C}}(x)$ iff $z \in \mathcal{T}_{\Psi_{i}}(x)$. It therefore suffices to compute $\mathcal{T}_{\mathcal{C}}(x)$ for $x \in D_{i}$.
Define $\overline{\mathcal{X}}_{0}(\mathbf{S}) = \overline{\mathcal{X}}(\mathbf{S}) \cap \mathcal{D}$. We will first show that,  for all $x$ with $b(x) = 0$, 
\begin{equation}
\label{eq:tangent-cone-equality}
\mathcal{T}_{\mathcal{D}}(x) = \bigcup_{\mathbf{S} \in \mathbf{S}(\mathbf{x})}{\mathcal{T}_{\overline{\mathcal{X}}_{0}(\mathbf{S})}(x)}.
\end{equation}
We observe that $$\mbox{dist}\left(x, \mathcal{D} \setminus \bigcup_{\mathbf{S} \in \mathbf{S}(x)}{\overline{\mathcal{X}}_{0}(\mathbf{S})}\right) > 0,$$ and hence $$\mbox{dist}(x+\tau z, \mathcal{D}) = \min_{\mathbf{S} \in \mathbf{S}(x)}{\mbox{dist}(x+\tau z,\overline{\mathcal{X}}_{0}(\mathbf{S}))}$$ for $\tau$ sufficiently small.

Suppose that $z \in \mathcal{T}_{\overline{\mathcal{X}}_{0}(\mathbf{S})}(x)$. Then for any $\tau \geq 0$, $\mbox{dist}(x + \tau z, \mathcal{D}) \leq \mbox{dist}(x + \tau z, \overline{\mathcal{X}}_{0}(\mathbf{S}))$ since $\overline{\mathcal{X}}_{0}(\mathbf{S}) \subseteq \mathcal{D}$, and hence $$\liminf_{\tau \rightarrow 0}{\frac{\mbox{dist}(x + \tau z, \mathcal{D})}{\tau}} \leq \liminf_{\tau \rightarrow 0}{\frac{\mbox{dist}(x + \tau z, \overline{\mathcal{X}}_{0}(\mathbf{S}))}{\tau}} = 0.$$  We therefore have $z \in \mathcal{T}_{\mathcal{D}}(x)$. 

Now, suppose that $z \in \mathcal{T}_{\mathcal{D}}(\mathbf{x})$ and yet $z \notin \bigcup_{\mathbf{S} \in \mathbf{S}(x)}{\mathcal{T}_{\overline{\mathcal{X}}_{0}(\mathbf{S})}(x)}$. 
Then for all $\mathbf{S} \in \mathbf{S}(x)$, there exists $\epsilon_{\mathbf{S}} > 0$ such that $$\liminf_{\tau \rightarrow 0}{\frac{\mbox{dist}(x + \tau z, \overline{\mathcal{X}}_{0}(\mathbf{S}))}{\tau}} = \epsilon_{\mathbf{S}}.$$ Let $\overline{\epsilon} = \min{\{\epsilon_{\mathbf{S}} : \mathbf{S} \in \mathbf{S}(x)\}}$. For any $\delta \in (0,\overline{\epsilon})$, there exists $\overline{\tau} > 0$ such that $\tau < \overline{\tau}$ implies 
\begin{displaymath}
\frac{\mbox{dist}(x + \tau z, \mathcal{D})}{\tau} = \min_{\mathbf{S} \in \mathbf{S}(x)}{\frac{\mbox{dist}(x + \tau z, \overline{\mathcal{X}}_{0}(\mathbf{S}))}{\tau}} 
> \delta
\end{displaymath}
implying that $\liminf_{\tau \rightarrow 0}{\frac{\mbox{dist}(x+\tau z, \mathcal{D})}{\tau}} > 0$ and hence $z \notin \mathcal{T}_{\mathcal{D}}(x)$. This contradiction implies (\ref{eq:tangent-cone-equality}).

It now suffices to show that, for each $\mathbf{S} \in \mathbf{S}(x)$, 
\begin{multline*}
\mathcal{T}_{\overline{\mathcal{X}}_{0}(\mathbf{S})}(x) = \left(\bigcap_{(i,j) \in \mathbf{T}(x) \cap \mathbf{S}}{\{z : (\overline{\mathbf{W}}_{i-1}(\mathbf{S})W_{ij})^{T}z \geq 0\}}\right) \cap \\ \left(\bigcap_{(i,j) \in \mathbf{T}(x) \setminus \mathbf{S}}{\{z : (\overline{\mathbf{W}}_{i-1}(\mathbf{S})W_{ij})^{T}z \leq 0\}}\right) 
\cap \{z : \overline{W}(\mathbf{S})^{T}z \geq 0\}.
\end{multline*}
We have that each $\overline{\mathcal{X}}_{0}(\mathbf{S})$ is given by 
\begin{multline*}
\overline{\mathcal{X}}_{0}(\mathbf{S}) = \{x^{\prime} : (\overline{\mathbf{W}}_{i-1}(\mathbf{S})W_{ij})^{T}x^{\prime} + r_{ij}(\mathbf{S}) \geq 0 \ \forall (i,j) \in \mathbf{S}\} \\
\cap \{x^{\prime} : (\overline{\mathbf{W}}_{i-1}(\mathbf{S})W_{ij})^{T}x^{\prime} + r_{ij}(\mathbf{S}) \leq 0 \ \forall (i,j) \notin \mathbf{S}\} \cap \{x^{\prime} : \overline{W}(\mathbf{S})^{T}x^{\prime} + r(\mathbf{S}) \geq 0\},
\end{multline*}
thus matching the conditions of Lemma \ref{lemma:TC-special} when each $g_{k}$ function is affine. Furthermore, the set $J(x)$ is equal to the set of functions that are exactly zero at $x$, which consists of $\{(\overline{\mathbf{W}}_{i-1}(\mathbf{S})W_{ij})^{T}x + \overline{r}_{ij}(\mathbf{S}) : (i,j) \in T(\mathbf{x})\}$ together with $\overline{W}(\mathbf{S})^{T}x + \overline{r}(\mathbf{S})$. This observation combined with Lemma \ref{lemma:TC-special} gives the desired result.
\end{proof}

% The following result is a consequence of Proposition \ref{lemma:tangent-cone-NN}.

Lemma \ref{lemma:NN-invariant} is a consequence of Proposition \ref{lemma:tangent-cone-NN}. For ease of exposition, we first reproduce the lemma and then present the proof.

\begin{lemma}
%\label{lemma:NN-invariant}
The set $\mathcal{D}$ is positive invariant if and only if, for all $x \in \partial \mathcal{D}$, there exist $\mathbf{S} \in \mathbf{S}(x)$ and $u \in \mathcal{U}$ satisfying 
\begin{align}
%\label{eq:safety-ineq-1}
(\overline{\mathbf{W}}_{i-1}(\mathbf{S})W_{ij})^{T}(f(x) + g(x)u) &\geq  0 \ \forall (i,j) \in \mathbf{T}(x) \cap \mathbf{S} \\
(\overline{\mathbf{W}}_{i-1}(\mathbf{S})W_{ij})^{T}(f(x)+g(x)u)&\leq 0 \ \forall (i,j) \in \mathbf{T}(x) \setminus \mathbf{S} \\
(\overline{\mathbf{W}}_{i-1}(\mathbf{S})W_{ij})^{T}(f(x) + g(x)u) &\geq 0 
\end{align}
\end{lemma}

%The proof follows immediately from Theorem \ref{theorem:Nagumo} and the proof of Proposition \ref{lemma:tangent-cone-NN} and is omitted due to space constraints. Based on Lemma \ref{lemma:curve-boundary-intersection} and Proposition \ref{lemma:tangent-cone-NN}, we now give an equivalent condition for avoiding each unsafe region.

 \begin{proof}
 By Theorem \ref{theorem:Nagumo}, the set $\mathcal{D}$ is positive invariant if and only if for every $x \in \partial \mathcal{D}$, there exists $u$ such that $(f(x) + g(x)u) \in \mathcal{T}_{\mathcal{D}}(x)$. By Proposition \ref{lemma:tangent-cone-NN}, this condition holds iff there exists $\mathbf{S} \in \mathbf{S}(x)$ such that 
\begin{multline*}
    (f(x)+g(x)u) \in \left(\left(\bigcap_{(i,j) \in \mathbf{T}(x) \cap \mathbf{S}}{\{z: (\overline{\mathbf{W}}_{i-1}(\mathbf{S})W_{ij})^{T}z \geq 0\}}\right) \cap \right.  \\
    \left. \left(\bigcap_{(i,j) \in \mathbf{T}(x) \setminus \mathbf{S}}{\{z : (\overline{\mathbf{W}}_{i-1}(\mathbf{S})W_{ij})^{T}z \leq 0\}}\right)
    \cap  \{z : \overline{W}(\mathbf{S})^{T}z \geq 0\}\right)
\end{multline*}
The above condition is equivalent to the conditions of the lemma, completing the proof.
 \end{proof}

%Authors may wish to optionally include extra information (complete proofs, additional experiments and plots) in the appendix. All such materials should be part of the supplemental material (submitted separately) and should NOT be included in the main submission.

\subsection{Proof of Proposition \ref{prop:safety-condition}}
\label{proof:prop:safety-condition}

% We first show that 

%Suppose that $x_{1} \in U_{i} \cap \mathcal{C}_{0}$. By Assumption \ref{assump:subset}, there exists $x_{2} \in U_{i} \setminus \mathcal{C}_{0} \subseteq \Phi_{i}$. Since $U_{i}$ is connected, there is a path from $x_{1} \notin \Psi_{i}$ to $x_{2} \in \Psi_{i}$ that is contained in $U_{i}$. Hence this path must cross the boundary of $\Psi_{i}$, which is equal to $D_{i}$, and we have $D_{i} \cap U_{i} \neq \emptyset$. Equivalently, if (ii) holds, then $U_{i} \cap \mathcal{C}_{0} = \emptyset$. 

First, suppose  that condition (i) holds. Then for any $x \in \mathcal{D}$ with $\mathbf{S}(x) = \{\mathbf{S}_{1},\ldots,\mathbf{S}_{r}\}$, there exists $l \in \{1,\ldots,r\}$ and $u \in \mathcal{U}$ such that $x \in \overline{\mathcal{X}}(\mathbf{S}_{l})$ and  (\ref{eq:safety-ineq-1})--(\ref{eq:safety-ineq-2}) hold. For this choice of $u$, we have $(f(x) + g(x)u) \in \mathcal{T}_{\Psi_{i}}(x)$ by Proposition \ref{lemma:tangent-cone-NN}. Hence $\mathcal{D}$ is positive invariant under any control policy consistent with $b$ by Lemma \ref{lemma:NN-invariant}.

Next, suppose that condition (ii) holds. Since $\mathcal{D}$ is contained in the union of the activation sets $\overline{\mathcal{X}}(\mathbf{S})$, this condition implies that $\mathcal{D} \subseteq \mathcal{C}$. 

\subsection{Proof of Lemma \ref{lemma:single-activation-set-condition}}
\label{proof:lemma:single-activation-set-condition}

 %We first show that, if condition (ii) holds, then $U_{i} \cap \mathcal{C}_{0} = \emptyset$, and hence $U_{i} \subseteq \Phi_{i}$. We then show that (i) implies that $\Psi_{i}$ is positive invariant, and hence the trajectory never reaches $\Phi_{i}$. 

%Suppose that $x_{1} \in U_{i} \cap \mathcal{C}_{0}$. By Assumption \ref{assump:subset}, there exists $x_{2} \in U_{i} \setminus \mathcal{C}_{0} \subseteq \Phi_{i}$. Since $U_{i}$ is connected, there is a path from $x_{1} \notin \Psi_{i}$ to $x_{2} \in \Psi_{i}$ that is contained in $U_{i}$. Hence this path must cross the boundary of $\Psi_{i}$, which is equal to $D_{i}$, and we have $D_{i} \cap U_{i} \neq \emptyset$. Equivalently, if (ii) holds, then $U_{i} \cap \mathcal{C}_{0} = \emptyset$. 

Suppose  that condition 1 holds. Then for any $x \in \partial \mathcal{D}$ with $\mathbf{S}(x) = \{\mathbf{S}_{1},\ldots,\mathbf{S}_{r}\}$, there exists $l \in \{1,\ldots,r\}$ such that $x \in \overline{\mathcal{X}}(\mathbf{S}_{l})$ and $u \in \mathcal{U}$ satisfy (\ref{eq:safety-ineq-1}) and (\ref{eq:safety-ineq-2}). For this choice of $u$, we have $(f(x) + g(x)u) \in \mathcal{T}_{\mathcal{D}}(x)$ by Proposition \ref{lemma:tangent-cone-NN}. Hence $\mathcal{D}$ is positive invariant under any control policy consistent with $b$ by Theorem \ref{theorem:Nagumo}. 
%We then have positive invariance of $\Psi_{i}$ by Theorem \ref{theorem:Nagumo} and Proposition \ref{lemma:tangent-cone-NN}. 

If Condition 2 holds, then there is no $x$ with $b(x) = 0$ and $x \in \mbox{int}(\overline{\mathcal{X}}(\mathbf{S}))$ such that $x \notin \mathcal{C}$. Hence, there are no counterexamples to condition (ii) of Proposition \ref{prop:safety-condition}.

\subsection{Proof of Lemma \ref{lemma:multi-activation-set-condition}}
\label{proof:lemma:multi-activation-set-condition}

The approach is to prove that condition (ii) of Proposition \ref{prop:safety-condition} holds; condition (i) holds automatically if each $\mathbf{S}_{1},\ldots,\mathbf{S}_{r}$ satisfies condition (ii) of Lemma \ref{lemma:single-activation-set-condition}. We have that conditions (a) and (b) are equivalent to $b(x) = 0$ and (\ref{eq:safety-condition-x}). In order for $x$ to be a safety counterexample, for all $l=1,\ldots,r$, at least one of Eqs. (\ref{eq:safety-ineq-1}) and (\ref{eq:safety-ineq-2}) must fail. Equivalently, for all $l=1,\ldots,r$, there does not exist $u$ satisfying
\begin{eqnarray*}%{rCl}
-(\overline{\mathbf{W}}_{i-1}(\mathbf{S}_{l})W_{ij})^{T}g(x)u &\leq& (\overline{\mathbf{W}}_{i-1}(\mathbf{S}_{l})W_{ij})^{T}f(x)  \ \forall (i,j) \in T(\mathbf{S}_{1},\ldots,\mathbf{S}_{r}) \cap \mathbf{S}_{l}\\
-(\overline{\mathbf{W}}_{i-1}(\mathbf{S}_{l})W_{ij})^{T}g(x)u &\geq& (\overline{\mathbf{W}}_{i-1}(\mathbf{S}_{l})W_{ij})^{T}f(x)  \ \forall (i,j) \in T(\mathbf{S}_{1},\ldots,\mathbf{S}_{r}) \setminus \mathbf{S}_{l} \\
-\overline{W}_{ij}(\mathbf{S}_{l})^{T}g(x)u &\leq& \overline{W}(\mathbf{S}_{l})^{T}f(x) \\
Au &\leq& c
\end{eqnarray*}
By Farkas Lemma, non-existence of such a $u$ is equivalent to existence of $y_{l}$ satisfying $y_{l} \geq 0$ as well as (\ref{eq:multiple-set-1}) and (\ref{eq:multiple-set-2}).

\subsection{Proof of Theorem \ref{theorem:overall-verification-proof}}
\label{proof:theorem:overall-verification-proof}
Suppose that $x$ is a safety counterexample for the NCBF $b$ with $b(x) = 0$. If $x \in \mbox{int}\overline{\mathcal{X}}(\mathbf{S})$ for some $\mathbf{S}$, then we have that $\mathbf{S} \in \mathcal{S}$ and hence a contradiction with Lemma \ref{lemma:single-activation-set-condition}. If $x \in \overline{\mathcal{X}}(\mathbf{S}_{1}) \cap \cdots \overline{\mathcal{X}}(\mathbf{S}_{r})$ for some $\mathbf{S}_{1},\ldots,\mathbf{S}_{r}$, then there is a contradiction with Lemma \ref{lemma:multi-activation-set-condition}. 

\subsection{Details on the IBP Procedure}
\label{sup:enumeration}
Interval bound propagation aims to compute an interval of possible output values by propagating a range of inputs layer-by-layer, and is integrated into our approach as follows. We first use partition the state space into cells and, for each cell, use LiRPA to derive upper and lower bounds on the value of b(x) when x takes values in that cell. When the interval of possible b(x) values in a cell contains zero, we conclude that that cell may intersect the boundary b(x) = 0. For each neuron, we use IBP to compute the pre-activation input interval for values of x within the cell. When the pre-activation input has a positive upper bound and negative lower bound, we identify the neuron as unstable, i.e., it may be either positive or negative for values of $x$ within the cell. Using this approach, we enumerate a collection of activation sets $\mathcal{S}$. We then identify the activation sets $\mathbf{S} \in \tilde{\mathcal{S}}$ such that $b(x) = 0$ for some $x \in \overline{\mathcal{X}}(\mathbf{S})$ by searching for an $x$ that satisfies the linear constraints in (16). This approach uses LiRPA and IBP to identify the activation regions that intersect the boundary $\{x: b(x) = 0\}$ without enumerating and checking all possible activation sets, which would have exponential runtime in the number of neurons in the network.

\subsection{Nonlinear Programming}
\label{subsec:nonlinear_prog}
The condition 2 of Lemma \ref{lemma:single-activation-set-condition} suffices to solve the nonlinear program
\begin{equation}
\label{eq:containment-verification}
\begin{array}{ll}
\mbox{minimize} & h(x) \\
\mbox{s.t.} & \overline{W}_{ij}(\mathbf{S})^{T}x + \overline{r}_{ij}(\mathbf{S}) \geq 0 \ \forall (i,j) \in \mathbf{S} \\
& \overline{W}_{ij}(\mathbf{S})^{T}x + \overline{r}_{ij}(\mathbf{S}) \leq 0 \ \forall (i,j) \notin \mathbf{S} \\
& \overline{W}(\mathbf{S})^{T}x + \overline{r}(\mathbf{S}) = 0
\end{array}
\end{equation}
and check whether the optimal value is nonnegative (unsafe) or negative (safe).

The verification problem of Lemma \ref{lemma:multi-activation-set-condition} can then be mapped to solving the nonlinear program
\begin{equation}
\label{eq:multiple-set-nonlinear-program}
\begin{array}{ll}
\mbox{min}_{x,y_{1},\ldots,y_{r}} & \max_{l=1,\ldots,r}{\left\{y_{l}^{T}\Lambda_{l}(\mathbf{S}_{1},\ldots,\mathbf{S}_{r},x)\right\}} \\
\mbox{s.t.} & (\overline{\mathbf{W}}_{i-1}(\mathbf{S}_{1})W_{ij})^{T}x + \overline{r}_{ij}(\mathbf{S}_1) < 0 \ \forall (i,j) \notin S_{1} \cup \cdots \cup S_{r} \\
& (\overline{\mathbf{W}}_{i-1}(\mathbf{S}_{1})W_{ij})^{T}x + \overline{r}_{ij}(\mathbf{S}_{1}) > 0 \ \forall (i,j) \in S_{1} \cap \cdots \cap S_{r} \\
& (\overline{\mathbf{W}}_{i-1}(\mathbf{S}_{1})W_{ij})^{T}x + \overline{r}_{ij}(\mathbf{S}_{1}) = 0 \ \forall (i,j) \in \mathbf{T}(\mathbf{S}_{1},\ldots,\mathbf{S}_{r}) \\
& y_{l}^{T}\Theta_{l}(\mathbf{S}_{1},\ldots,\mathbf{S}_{r}(x)) = 0 \ \forall l=1,\ldots,r \\
& y_{l} \geq 0 \ \forall l=1,\ldots,r
\end{array}
\end{equation}
and checking whether the optimal value is nonnegative (safe) or negative (unsafe). 
\input{sections/Experiment_Supplimentary}
